# Supplementary material for: Symmetry-Breaking Magneto-Optical Effects in Altermagnets
Source: arXiv:2505.24124 ancillary file (2025-05-30)
Supplement: Supplementary file 1 [file SI.pdf]

# Supplemental Information for: Symmetry-Breaking Magneto-Optical Effects in Altermagnets

Jiuyu Sun, Yongping Du,* and Erjun Kan†
*Department of Applied Physics, Nanjing University of Science and Technology, Nanjing 210094, China and MIIT Key Laboratory of Semiconductor Microstructure and Quantum Sensing, Nanjing University of Science and Technology, Nanjing 210094, China*
(Dated: May 30, 2025)

## I. COMPUTATIONAL METHODOLOGY

### A. Computational parameters

Our density functional theory calculations were performed using the Quantum Espresso package[1, 2] with the optimized norm-conserving Vanderbilt pseudopotentials[3, 4]. All the optical properties are computed using Yambo code with the spin-orbit coupling effect included unless specific clarification.

For $V_2Se_2O$ monolayer, the geometric structure of were fully relaxed with the PBE[5] functional and a cutoff energy of 90 Ry for the planewave basis. The lattice constant was optimized to be 3.88 Å, which is in agreement with previous works[6–8]. For the quasiparticle band structures, we adopted the band structures and wavefunctions by PBE+$U$ with $U_{\text{eff}} = 4.5$ eV. Note, to mimics the self-energy effect to the quasi-particle bands, we applied a scissor operator of 2.0 eV to the PBE+U ground state wavefunction as the starting point of all the many-body perturbation calculations. The reason to choosing this scissor operator has been discussed in our previous work[9]. All the spin-resolved many-body perturbation calculations[10–13] were performed by using Yambo package[14, 15] with a Γ-centered k-mesh of $16 \times 16 \times 1$. The static dielectric matrix are calculated via the random-phase approximation (RPA) with 360 bands and a 12 Ry cutoff. With this static dielectric screening, the optical properties are obtained by solving the Bethe-Salpeter equation (BSE) with 14 pairs of valence and conduction bands. The convergence tests of the computational parameters can also be found in our previous work[9].

For the CrSb bulk, the experimental lattice constants ($a = b = 4.1243$ Å, $c = 5.4728$ Å) were used. A cutoff energy of 100 Ry for the plane-wave basis and a Γ-centered k-mesh $18 \times 18 \times 11$ are used for calculating the self-consistent ground state and optical properties. Due to the metallic nature, we did not consider the excitonic effects, and the optical properties are computed within independent-particle picture with 12 pairs of valence and conduction bands near the Fermi level. For the MnTe bulk below, we applied the same computational method and parameters, with its experimental lattice constants ($a = b = 4.14$ Å, $c = 6.71$ Å)[16].

### B. Formula for MOKE in 2D monolayer

From Ref. [17], we simply borrow the formula for calculating the MOKE signal in a 2D monolayer with a semi-infinite substrate. In the presence of a magnetization along the $z$-axis and spin–orbit coupling, the effective dielectric tensor of $V_2Se_2O$ assumes the form

$$\varepsilon = \begin{pmatrix} \varepsilon_{xx} & \varepsilon_{xy} & 0 \\ -\varepsilon_{xy} & \varepsilon_{xx} & 0 \\ 0 & 0 & \varepsilon_{zz} \end{pmatrix}. \tag{1}$$

Then the Kerr angle can be derived as

$$\theta_{\text{K}} = -\frac{1}{2} \arg \left( \frac{r_+}{r_-} \right), \tag{2}$$

* dypnjust@njust.edu.cn.
† ekan@njust.edu.cn

where $r_\pm$ are the reflection coefficients, given by

$$r_\pm = \frac{1 - n_\mp h(n_\mp)}{1 + n_\mp h(n_\mp)}, \tag{3}$$

in which $n_\pm = \sqrt{\varepsilon_{xx} \pm i\varepsilon_{xy}}$ are the refractive indexes in the circular basis and

$$h(n_\pm) = \frac{f(n_\pm) - g(n_\pm)}{f(n_\pm) + g(n_\pm)}, \tag{4}$$

$$f(n_\pm) = (n_\pm + \sqrt{\varepsilon_\mathrm{r}})\mathrm{e}^{-\mathrm{i}\frac{\omega}{c}n_\pm d},\ g(n_\pm) = (n_\pm - \sqrt{\varepsilon_\mathrm{r}})\mathrm{e}^{\mathrm{i}\frac{\omega}{c}n_\pm d}. \tag{5}$$

Here, $\varepsilon_\mathrm{r}$ is the relative permittivity of a $SiO_2$ substrate, which is set to 2.4 as in Ref. [17]. In this way, with the dielectric matrix ($\varepsilon_{xx}$ and $\varepsilon_{xy}$) calculated from first-principles, we simulate the polar MOKE in $V_2Se_2O$ monlayer.

## II. MORE RESULTS FOR CRSB

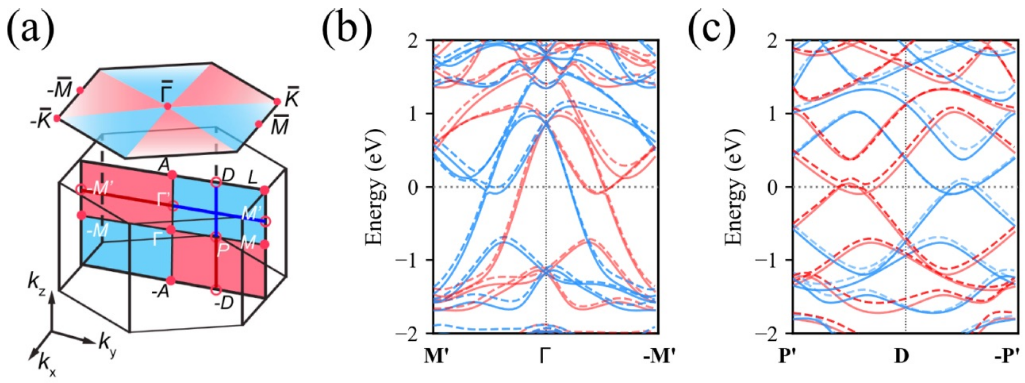


FIG. 1. (a) The top-view and side-view of strained crystal structure of MnTe, where the red (blue) arrows on Mn1 (Mn2) atoms indicate the direction of their magnetic moments. Within (c) $xy$-plane and (d) $xz$-plane, strain-dependent Kerr rotation angle $\theta_K$.

## III. RESULTS FOR MNTE

We study the hexagonal MnTe, as an additional example for the semiconducting bulks. Reported in previous works[18–20], MnTe has a Neel vector along [110] direction, with the spin-up and spin-down octahedrons are connected by a $C_{6z}$ rotation and a $M_z$ mirror. Due to the anti-symmetry character of $\sigma_{xy}$, it could be non-zero under the $M_z$ operation, i.e. $M_z(\sigma_{zy}, \sigma_{xz}, \sigma_{yx}) = (-\sigma_{zy}, -\sigma_{xz}, \sigma_{yx})$. Thus, the non-zero $\sigma_{xy}$ results in an intrinsic MOKE rotation within $xy$-plane (Figure 2b), while other two vanishing components $\sigma_{xz}$ and $\sigma_{yz}$ prohibit the presence of MOKE signal within $yz$- and $xz$-planes (Figure 2c). On the other hand, considering the crystal orientation of an arbitrary sample grown on a substrate cannot be easily controlled in practice, the polar MOKE measurement is still likely to be zero if the polarization of probe light is in $xz$- or $yz$-plane.

To overcome this limitation, a uniaxial strain with the direction along neither $C_{6z}$ axis nor $xy$-plane should be working. Here, we choose a strain along [111] direction, which is simulated by canting the lattice vector $\boldsymbol{c}$ slightly towards [110], with the angle ($\varphi$) between lattice vector $\boldsymbol{a}(\boldsymbol{b})$ from 90° to 87° with a step of 1°. As demonstrated in Figure 2(a), this uniaxial strain non-equivalently tilts the spin-up (red) and spin-down (blue) octahedrons, in which the $d_{z^2}$ orbitals of Mn1 and Mn2 atoms are stretched and compressed, respectively. Consequently, for the strained MnTe, we found not only the enhanced MOKE within $xy$-plane, but also the appearance of MOKE signal within

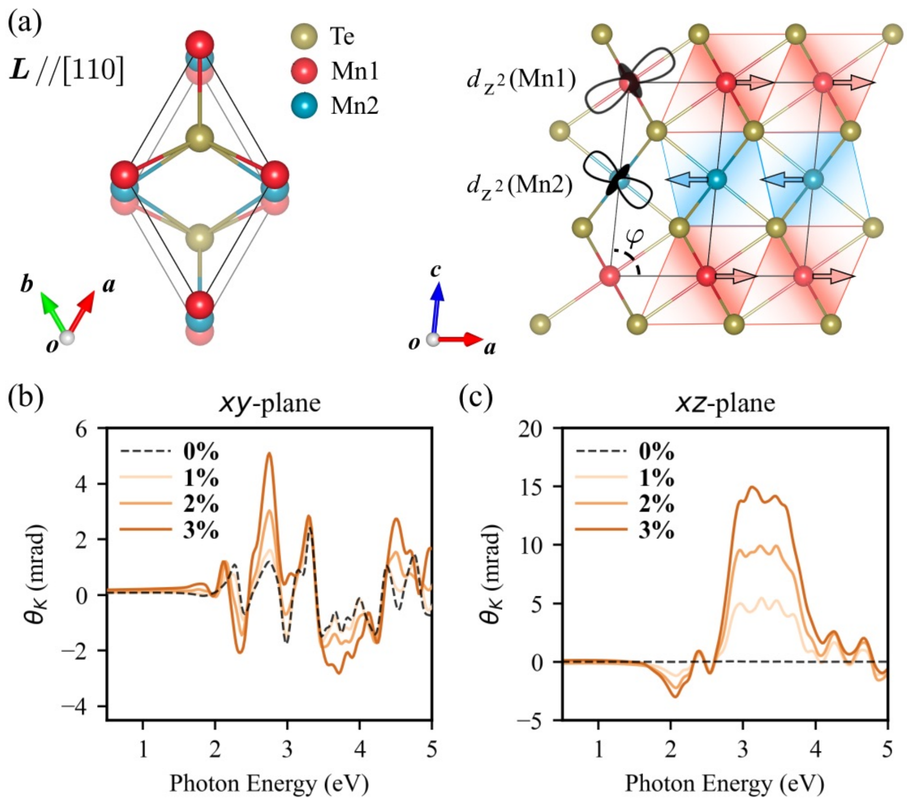


FIG. 2. (a) The top-view and side-view of strained crystal structure of MnTe, where the red (blue) arrows on Mn1 (Mn2) atoms indicate the direction of their magnetic moments. Within (c) $xy$-plane and (d) $xz$-plane, strain-dependent Kerr rotation angle $\theta_K$.

$xz$-plane with even larger $\theta_K$ than that within $xy$-plane.


[1] P. Giannozzi, S. Baroni, N. Bonini, M. Calandra, R. Car, C. Cavazzoni, D. Ceresoli, G. L. Chiarotti, M. Cococcioni, I. Dabo, A. Dal Corso, S. de Gironcoli, S. Fabris, G. Fratesi, R. Gebauer, U. Gerstmann, C. Gougoussis, A. Kokalj, M. Lazzeri, L. Martin-Samos, N. Marzari, F. Mauri, R. Mazzarello, S. Paolini, A. Pasquarello, L. Paulatto, C. Sbraccia, S. Scandolo, G. Sclauzero, A. P. Seitsonen, A. Smogunov, P. Umari, and R. M. Wentzcovitch, Quantum espresso: a modular and open-source software project for quantum simulations of materials, J. Phys. Condens. Matter **21**, 395502 (2009).

[2] P. Giannozzi, O. Andreussi, T. Brumme, O. Bunau, M. B. Nardelli, M. Calandra, R. Car, C. Cavazzoni, D. Ceresoli, M. Cococcioni, N. Colonna, I. Carnimeo, A. D. Corso, S. de Gironcoli, P. Delugas, R. A. D. Jr, A. Ferretti, A. Floris, G. Fratesi, G. Fugallo, R. Gebauer, U. Gerstmann, F. Giustino, T. Gorni, J. Jia, M. Kawamura, H.-Y. Ko, A. Kokalj, E. Küçükbenli, M. Lazzeri, M. Marsili, N. Marzari, F. Mauri, N. L. Nguyen, H.-V. Nguyen, A. O. de-la Roza, L. Paulatto, S. Poncé, D. Rocca, R. Sabatini, B. Santra, M. Schlipf, A. P. Seitsonen, A. Smogunov, I. Timrov, T. Thonhauser, P. Umari, N. Vast, X. Wu, and S. Baroni, Advanced capabilities for materials modelling with quantum espresso, Journal of Physics: Condensed Matter **29**, 465901 (2017).

[3] D. R. Hamann, Optimized norm-conserving vanderbilt pseudopotentials, Phys. Rev. B **88**, 085117 (2013).

[4] M. van Setten, M. Giantomassi, E. Bousquet, M. Verstraete, D. Hamann, X. Gonze, and G.-M. Rignanese, The pseudodojo: Training and grading a 85 element optimized norm-conserving pseudopotential table, Computer Physics Communications **226**, 39 (2018).

[5] J. P. Perdew, K. Burke, and M. Ernzerhof, Generalized gradient approximation made simple, Phys. Rev. Lett. **77**, 3865 (1996).

[6] H.-Y. Ma, M. Hu, N. Li, J. Liu, W. Yao, J.-F. Jia, and J. Liu, Multifunctional antiferromagnetic materials with giant piezomagnetism and noncollinear spin current, Nature Communications **12**, 2846 (2021).

[7] H. Lin, J. Si, X. Zhu, K. Cai, H. Li, L. Kong, X. Yu, and H.-H. Wen, Structure and physical properties of $CsV_2Se_{2-x}O$ and $V_2Se_2O$, Phys. Rev. B **98**, 075132 (2018).

[8] Y. Qi, J. Zhao, and H. Zeng, Spin-layer coupling in two-dimensional altermagnetic bilayers with tunable spin and valley

splitting properties, Physical Review B **110**, 14442 (2024).

[9] J. Sun, J. Han, Y. Du, and E. Kan, Optical controllable spin-polarization in two dimensional altermagnets via robust spin-momentum locking excitons, submitted (2025), arXiv:2505.23237.

[10] A. Castro, E. Räsänen, and C. A. Rozzi, Exact coulomb cutoff technique for supercell calculations in two dimensions, Phys. Rev. B **80**, 033102 (2009).

[11] M. Marsili, A. Molina-Sánchez, M. Palummo, D. Sangalli, and A. Marini, Spinorial formulation of the $GW$-BSE equations and spin properties of excitons in two-dimensional transition metal dichalcogenides, Phys. Rev. B **103**, 155152 (2021).

[12] M. Rohlfing and S. G. Louie, Electron-hole excitations and optical spectra from first principles, Phys. Rev. B **62**, 4927 (2000).

[13] L. X. Benedict and E. L. Shirley, Ab initio calculation of $\epsilon_2(\omega)$ including the electron-hole interaction: Application to gan and $caf_2$, Phys. Rev. B **59**, 5441 (1999).

[14] A. Marini, C. Hogan, M. Grüning, and D. Varsano, Yambo: an ab initio tool for excited state calculations, Comput. Phys. Commun. **180**, 1392 (2009).

[15] D. Sangalli, A. Ferretti, H. Miranda, C. Attaccalite, I. Marri, E. Cannuccia, P. Melo, M. Marsili, F. Paleari, A. Marrazzo, G. Prandini, P. Bonfà, M. O. Atambo, F. Affinito, M. Palummo, A. Molina-Sánchez, C. Hogan, M. Grüning, D. Varsano, and A. Marini, Many-body perturbation theory calculations using the Yambo code, J. Phys.: Condens. Matter **31**, 325902 (2019).

[16] D. Kriegner, H. Reichlova, J. Grenzer, W. Schmidt, E. Ressouche, J. Godinho, T. Wagner, S. Y. Martin, A. B. Shick, V. V. Volobuev, G. Springholz, V. Holý, J. Wunderlich, T. Jungwirth, and K. Výborný, Magnetic anisotropy in antiferromagnetic hexagonal mnte, Phys. Rev. B **96**, 214418 (2017).

[17] A. Molina-Sánchez, G. Catarina, D. Sangalli, and J. Fernández-Rossier, Magneto-optical response of chromium trihalide monolayers: chemical trends, J. Mater. Chem. C **8**, 8856 (2020), arXiv:1912.01888.

[18] J. Krempaský, L. Šmejkal, S. W. D'Souza, M. Hajlaoui, G. Springholz, K. Uhlířová, F. Alarab, P. C. Constantinou, V. Strocov, D. Usanov, W. R. Pudelko, R. González-Hernández, A. Birk Hellenes, Z. Jansa, H. Reichlová, Z. Šobáň, R. D. Gonzalez Betancourt, P. Wadley, J. Sinova, D. Kriegner, J. Minár, J. H. Dil, and T. Jungwirth, Altermagnetic lifting of Kramers spin degeneracy, Nature **626**, 517 (2024), arXiv:2308.10681.

[19] S. Lee, S. Lee, S. Jung, J. Jung, D. Kim, Y. Lee, B. Seok, J. Kim, B. G. Park, L. Šmejkal, C.-J. Kang, and C. Kim, Broken Kramers Degeneracy in Altermagnetic MnTe, Physical Review Letters **132**, 036702 (2024), arXiv:2308.11180.

[20] A. Hariki, A. Dal Din, O. J. Amin, T. Yamaguchi, A. Badura, D. Kriegner, K. W. Edmonds, R. P. Campion, P. Wadley, D. Backes, L. S. I. Veiga, S. S. Dhesi, G. Springholz, L. Šmejkal, K. Výborný, T. Jungwirth, and J. Kuneš, X-Ray Magnetic Circular Dichroism in Altermagnetic $\alpha$-MnTe, Physical Review Letters **132**, 176701 (2024), arXiv:2305.03588.
